# Supplementary material for: Single-laser feedback cooling of optomechanical resonators
Source: arXiv:2209.06029 source file (2022-09-28)

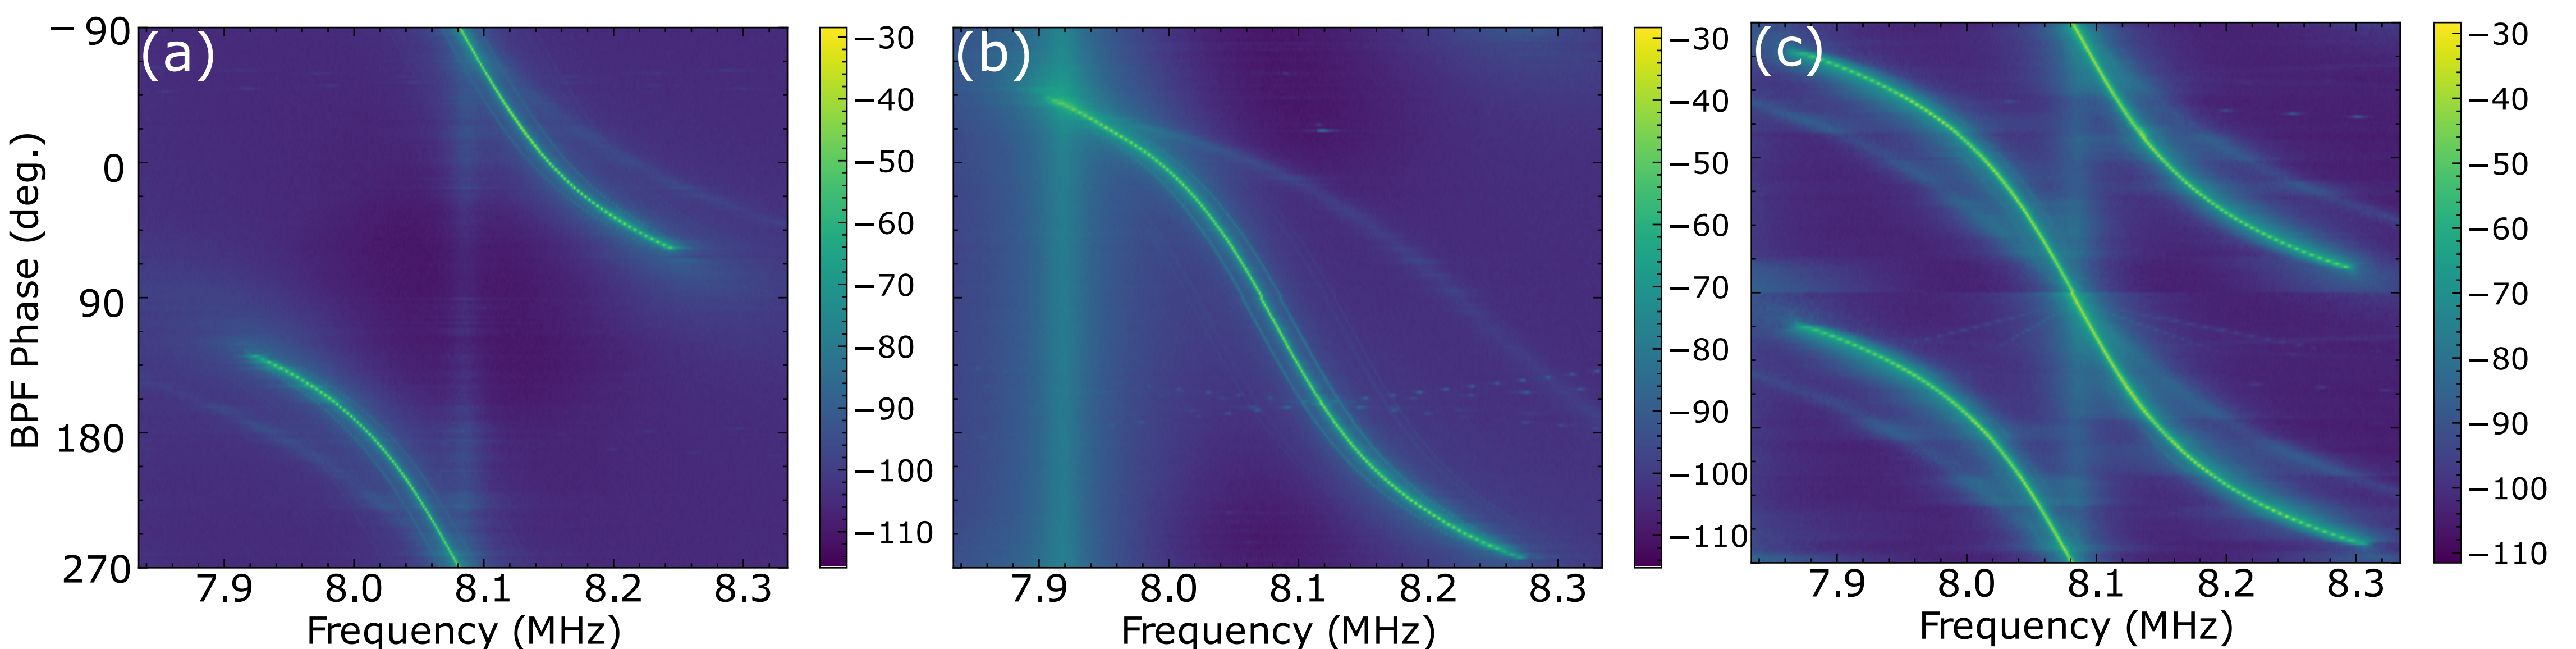

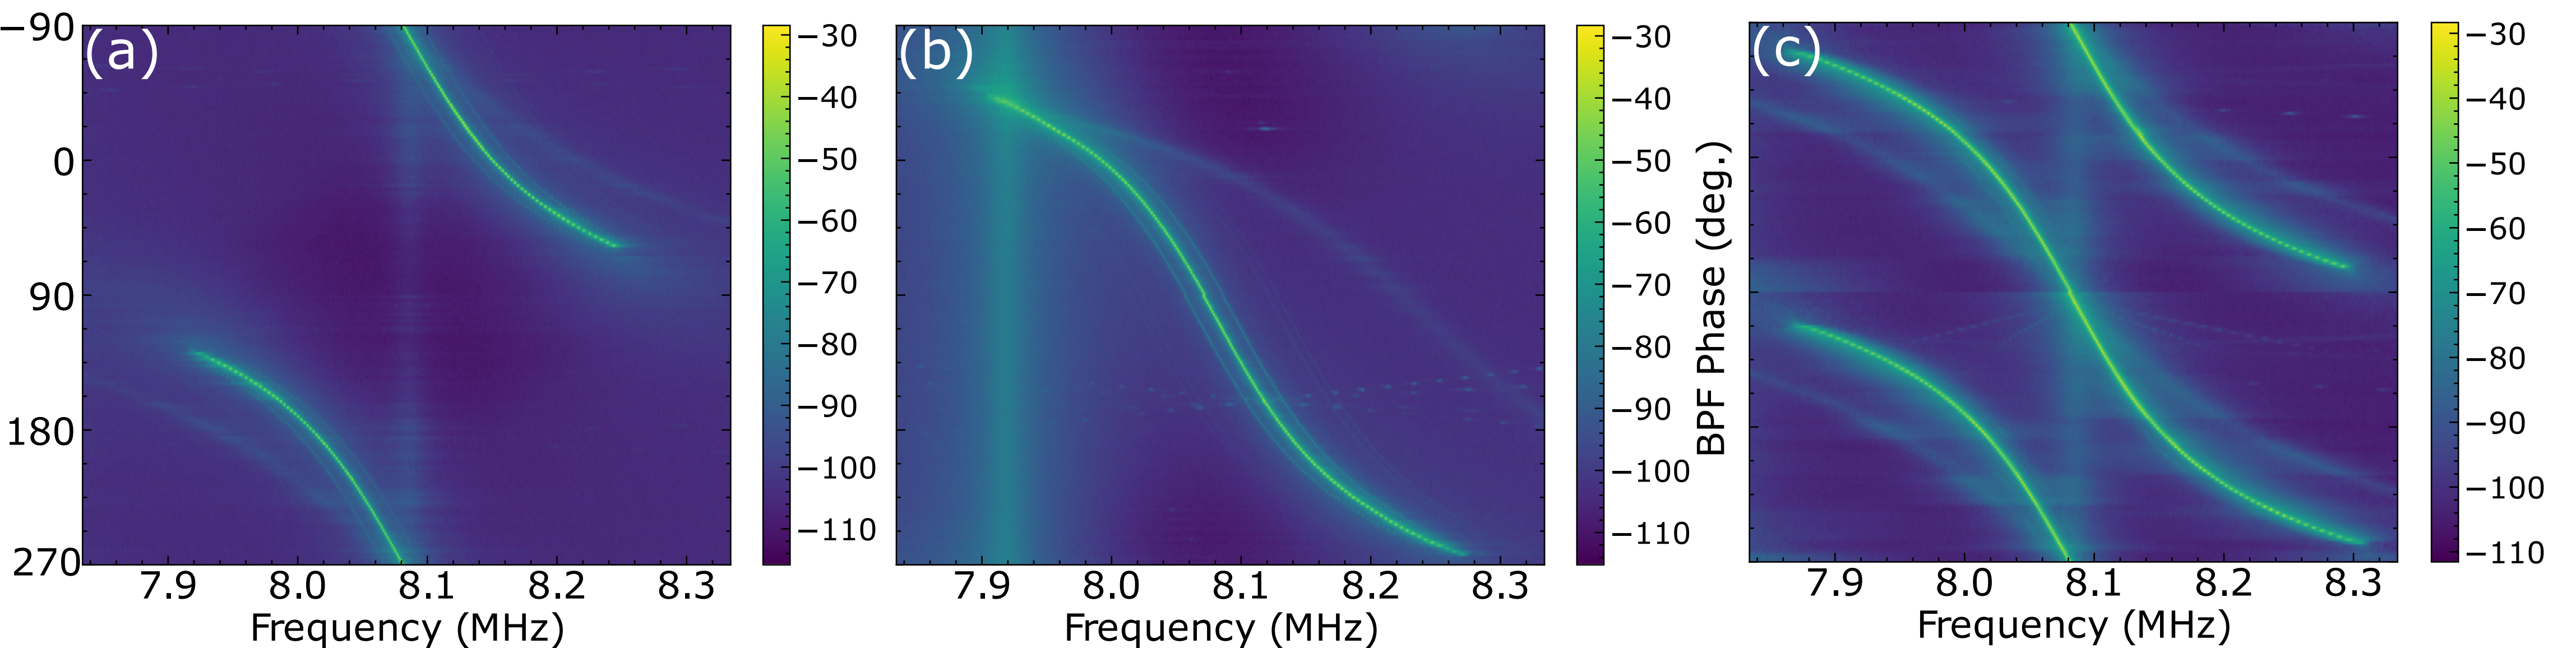

Supplement: Supplementary file 1 [file expt_scans_SM.pdf]
